# Supplementary material for: Optical shielding of destructive chemical reactions between ultracold ground-state NaRb molecules
Source: arXiv:2006.09014 source file (2020-08-12)
Supplement: Supplementary file 1 [file NaRb_SM.pdf]

# Supplementary Material for Optical shielding of destructive chemical reactions between ultracold ground-state NaRb molecules

T. Xie[1], M. Lepers[2], R. Vexiau[1], A. Orbán[3], O. Dulieu[1], and N. Bouloufa-Maafa[1]
[1] *Université Paris-Saclay, CNRS, Laboratoire Aimé Cotton, 91405 Orsay, France*
[2] *Laboratoire Interdisciplinaire Carnot de Bourgogne, CNRS, Université de Bourgogne Franche-Comté, 21078 Dijon, France and*
[3] *Institute for Nuclear Research, Hungarian Academy of Sciences(ATOMKI), H-4001 Debrecen, Pf. 51, Hungary*

PACS numbers:

## A. Long-range potential energy curves for two interacting $^{23}$Na$^{87}$Rb molecules

The computation of such potential energy curves (PECs) closely follows the procedure described in Ref. [1], using the properly symmetrized basis functions in the laboratory frame $|e_1, j_1, p_1, e_2, j_2, p_2, j_{12}, \ell, J, M\rangle|n\rangle$ introduced in the main text. Both molecules are assumed to be in the lowest vibrational level of the $e_1$ and $e_2$ electronic states, so that this quantum number is omitted in the following. The $e_1$ and $e_2$ states can either be the electronic ground state $X^1\Sigma^+$ or the lowest electronic excited long-lived state $b^3\Pi_0$ (respectively noted in short as $X$ and $b$ states).

In the absence of external electric field, the permanent dipole moment of the alkali-metal ground-state molecules (equal to 1.304 a.u. for the $v_X = 0$ level [2]) generates a strong dipole-dipole interaction (DDI) scaling as $R^{-3}$ at large distance between a molecule in $j_X = 0$ and another in $j_X = 1$. In contrast, two ($j_X = 0$) molecules interact at large distances trough a $-C_6^g/R^6$ term, with $C_6^g = 1.516\times10^6$ a.u. for $^{23}$Na$^{87}$Rb [3, 4]. This gigantic value is induced by the DDI at the second order of perturbation. The interaction also involves a second term $C_6^e$ coming from transitions toward excited electronic states of the two molecules, and a third term $C_6^{g-e}$ coming from the purely rotational transition ($j_X = 0 \to j_X = 1$) for one molecule and from transitions toward excited electronic states for the other. For $^{23}$Na$^{87}$Rb, $C_6^e = 7731$ a.u., while $C_6^{g-e} = 644$ a.u. [4]. We take the sum of these two terms as the van der Waals interaction coefficient $C_6^{\rm el}$ in the main text.

The long-range interaction between the ($j_X$) and the ($j_b$) levels is more complicated than in the previous case. The total DDI comes from two parts: (i) the direct interaction between the permanent dipole moments (PDMs) in the $X$ and $b$ states, and (ii) the resonant interaction between the $X$ and $b$ states, involving the corresponding transition dipole moments (PDMs) (just like in the well-known $S + P$ atom-atom long-range interaction). The relative strengths of these two types of interactions can be estimated by comparing the product of PDMs on the one hand, which gives 2.263 a.u., and the square of the TDM on the other hand, which gives $3.679 \times 10^{-2}$ a.u. (see Table III). However one should keep in mind that the two terms do not couple the same pairs of molecular levels. For example, the direct term couples the pairs ($j_X = 0, j_b = 1$) and ($j_X = 1, j_b = 0$), while the resonant one couples ($j_X = 0, j_b = 1$) with ($j_b = 1, j_X = 0$). In addition to these terms, there is the van der Waals term $-C_6^{\rm el}/R^6$ induced by virtual transitions toward other electronic states than $X$ and $b$, with an unknown value. Assuming a typical $C_6^{\rm el}$ coefficient of a few thousands of a.u., this term is significant only for distances smaller than the one where we start the log-derivative propagation ($R_{min} = 10$ a.u., ), so that it does not influence the calculations. Therefore for numerical purpose (see Section E), we take the same $C_6^{\rm el} = 8375$ a.u. as above, but we do not expect this value to have any influence on our results.

As $^{23}$Na$^{87}$Rb molecules are bosons, the scattering wave functions for a pair of $^{23}$Na$^{87}$Rb ($X$) molecules are symmetric upon the permutation of two molecules. Starting from a pair of ($j_X = 0$) molecules, the collision can only involve even partial waves $\ell$, so that the values of the total angular momentum quantum number are $J = 0, 2, 4, ...$ (since $j_{12} = 0$) and $M = 0$. The parity with respect to inversion of all coordinates, equal to $p_1p_2(-1)^\ell$, is also even. The states correlated to $^{23}$Na$^{87}$Rb($j_X = 0$)+$^{23}$Na$^{87}$Rb($j_X = 0$) are coupled by the laser to odd-parity states of the [$^{23}$Na$^{87}$Rb($j_X = 0$),$^{23}$Na$^{87}$Rb($j_b = 1$)] pair, itself coupled to [$^{23}$Na$^{87}$Rb($j_X = 1$),$^{23}$Na$^{87}$Rb($j_b = 0$)] by dipolar interaction, and again involving even partial waves.

The resulting adiabatic PECs (without light interaction) are drawn in Figures 1 and 2. We report in Tables I and II the corresponding basis sets correlated to the dissociation limits visible in the Figures. From the tables we can see that the states relevant to the thresholds presented in Figures 1 and 2 have $j$-values smaller than 2. To minimize the computation time without altering the precision, we examined the convergence of the coupled-channel results considering basis sets with different $j_{\rm max}$ and $\ell_{\rm max}$. Without laser field, we can reproduce the reactive rate coefficients observed in $^{23}$Na$^{87}$Rb experiment [5] with $j_{\rm max} = 2$ and $\ell_{\rm max} = 4$ since $j_1$ and $j_2$ are both equal to 0 in the lowest channel. In the presence of optical field, the exit channels with highest energy are ($j_X = 0$)+$b$($j_b = 1$), and we set $j_{\rm max} = 4$ and $\ell_{\rm max} = 4$ in the basis set for both ground and excited states. This results in 474 (resp. 329) coupled Schrödinger equations for $J = 0, 2$ (resp. $J = 1, 2, 3$) in the circular (resp. linear) polarization case.

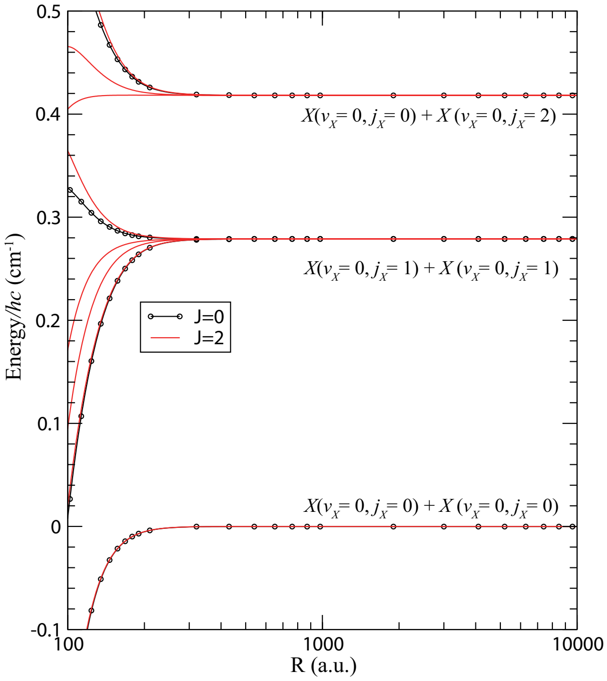


FIG. 1: The adiabatic long-range potential-energy curves of even parity (without light interaction) correlated to the dissociation limits $^{23}$Na$^{87}$Rb$(j_X)$+$^{23}$Na$^{87}$Rb$(j_X)$, assuming that both molecules are in their lowest vibrational level. Only partial waves $\ell = 0, 2, 4$ are included.

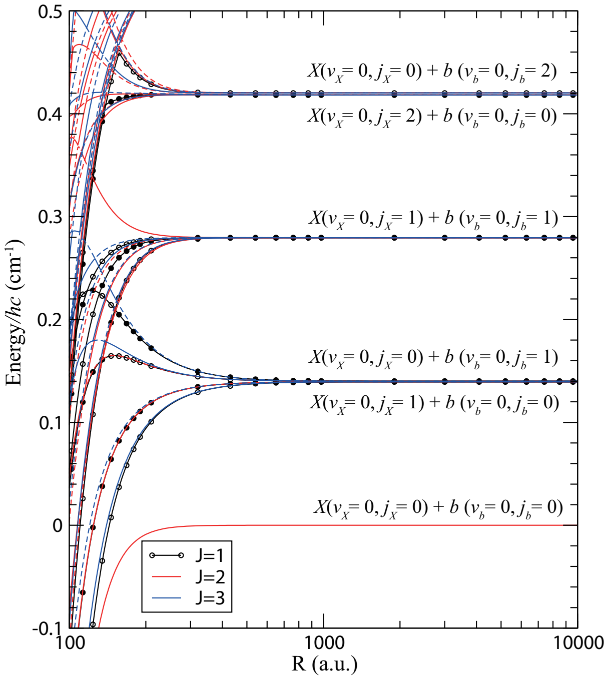


FIG. 2: The adiabatic long-range potential-energy curves of odd parity (without light interaction) correlated to the dissociation limits $^{23}$Na$^{87}$Rb$(j_X)$+$^{23}$Na$^{87}$Rb$(j_b)$, assuming that both molecules are in their lowest vibrational level. Only partial waves $\ell = 0, 2, 4$ are included.

| $j_1$ | $p_1$ | $j_2$ | $p_2$ | $j_{12}$ | $\ell$ | $J$ |
|---|---|---|---|---|---|---|
| 0 | 1 | 0 | 1 | 0 | 0 | 0 |
| 0 | 1 | 2 | 1 | 2 | 2 | 0 |
| 1 | -1 | 1 | -1 | 0 | 0 | 0 |
| 1 | -1 | 1 | -1 | 2 | 2 | 0 |
| 0 | 1 | 0 | 1 | 0 | 2 | 2 |
| 0 | 1 | 2 | 1 | 2 | 0 | 2 |
| 0 | 1 | 2 | 1 | 2 | 2 | 2 |
| 0 | 1 | 2 | 1 | 2 | 4 | 2 |
| 1 | -1 | 1 | -1 | 0 | 2 | 2 |
| 1 | -1 | 1 | -1 | 2 | 0 | 2 |
| 1 | -1 | 1 | -1 | 2 | 2 | 2 |
| 1 | -1 | 1 | -1 | 2 | 4 | 2 |

TABLE I: Basis vectors correlated to the dissociation limits $^{23}$Na$^{87}$Rb$(j_X)$+$^{23}$Na$^{87}$Rb$(j_X)$ displayed in Fig.1, restricted to $\ell = 0, 2, 4$ and $J = 0, 2$.

| $j_1$ | $p_1$ | $j_2$ | $p_2$ | $j_{12}$ | $\ell$ | $J$ |
|---|---|---|---|---|---|---|
| 0 | 1 | 1 | -1 | 1 | 0 | 1 |
| 0 | 1 | 1 | -1 | 1 | 2 | 1 |
| 0 | 1 | 2 | -1 | 2 | 2 | 1 |
| 1 | -1 | 0 | 1 | 1 | 0 | 1 |
| 1 | -1 | 0 | 1 | 1 | 2 | 1 |
| 1 | -1 | 1 | 1 | 1 | 0 | 1 |
| 1 | -1 | 1 | 1 | 1 | 2 | 1 |
| 1 | -1 | 1 | 1 | 2 | 2 | 1 |
| 2 | 1 | 0 | -1 | 2 | 2 | 1 |
| 0 | 1 | 0 | -1 | 0 | 2 | 2 |
| 0 | 1 | 1 | -1 | 1 | 2 | 2 |
| 0 | 1 | 2 | -1 | 2 | 0 | 2 |
| 0 | 1 | 2 | -1 | 2 | 2 | 2 |
| 0 | 1 | 2 | -1 | 2 | 4 | 2 |
| 1 | -1 | 0 | 1 | 1 | 2 | 2 |
| 1 | -1 | 1 | 1 | 0 | 2 | 2 |
| 1 | -1 | 1 | 1 | 1 | 2 | 2 |
| 1 | -1 | 1 | 1 | 2 | 0 | 2 |
| 1 | -1 | 1 | 1 | 2 | 2 | 2 |
| 1 | -1 | 1 | 1 | 2 | 4 | 2 |
| 2 | 1 | 0 | -1 | 2 | 0 | 2 |
| 2 | 1 | 0 | -1 | 2 | 2 | 2 |
| 2 | 1 | 0 | -1 | 2 | 4 | 2 |
| 0 | 1 | 1 | -1 | 1 | 2 | 3 |
| 0 | 1 | 1 | -1 | 1 | 4 | 3 |
| 0 | 1 | 2 | -1 | 2 | 2 | 3 |
| 0 | 1 | 2 | -1 | 2 | 4 | 3 |
| 1 | -1 | 0 | 1 | 1 | 2 | 3 |
| 1 | -1 | 0 | 1 | 1 | 4 | 3 |
| 1 | -1 | 1 | 1 | 1 | 2 | 3 |
| 1 | -1 | 1 | 1 | 1 | 4 | 3 |
| 1 | -1 | 1 | 1 | 2 | 2 | 3 |
| 2 | 1 | 0 | -1 | 2 | 2 | 3 |
| 2 | 1 | 0 | -1 | 2 | 4 | 3 |

TABLE II: Basis vectors correlated to the dissociation limits $^{23}$Na$^{87}$Rb$(X, j_X)$+$^{23}$Na$^{87}$Rb$(b, j_b)$ displayed in Fig.2, restricted to $\ell = 0, 2, 4$ and $J = 1, 2, 3$.

### B. Dressed potential energy curves between two $^{23}$Na$^{87}$Rb molecules in circular polarization

In complement to the Figure of the main text in the linear polarization case, we present in Fig. 3 the $^{23}$Na$^{87}$Rb-$^{23}$Na$^{87}$Rb dressed adiabatic long-range PECs in the pres-

ence of circularly-polarized laser field. The asymptotes are labeled with the approximated good quantum number $j_X$, $j_b$ and $n$. For circular polarization, an extra transition from $J = 2$ to $J' = 2$ is allowed, and two additional states correlated to the asymptotes $(j_X = 1) + (j_b = 0)$ and $(j_X = 0) + (j_b = 1)$ with $J = 2$ exist compared to the linear polarization case. As demonstrated in the main text, the circular light field is expected to generate a better shielding efficiency than the linear field. However, the global landscape of the PECs is very similar for both polarizations at the displayed scale. Note that the shifts of the asymptotes are identical for both polarizations.

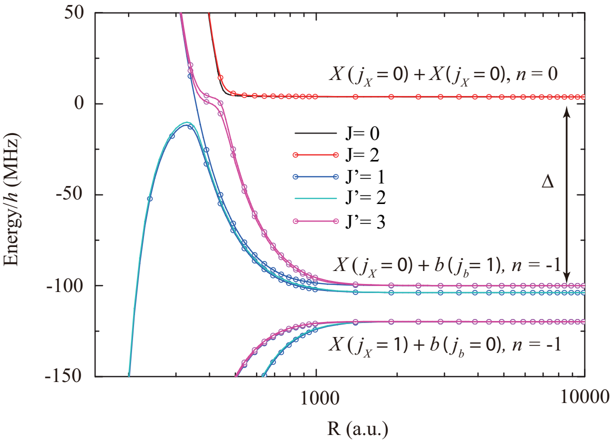


FIG. 3: The dressed adiabatic long-range potential-energy curves of $^{23}$Na$^{87}$Rb-$^{23}$Na$^{87}$Rb for $\Delta = 100$ MHz and $\Omega = 10$ MHz in circularly- polarized light field. The Condon point (not displayed here) lies around $R_C = 400$ a.u.. As in the linear polarization case, the asymptotic spacing between the $(j_X = 0) + (j_X = 0)$ and $(j_X = 0) + (j_b = 1)$ asymptotes is slightly larger than $\Delta$ due to the presence of the stationary laser field [6].

### C. About the hyperfine structure in the $b$ state

Ultracold molecule experiments rely on the creation of Feshbach molecules in the presence of a static magnetic field, as the first step of the of ultracold ground-state molecules. Therefore the role of the hyperfine structure (hfs) in the optical shielding must be discussed.

As stated in the main text, the hfs of the molecular states is neglected. The one of the $X$ state of $^{23}$Na$^{87}$Rb lies in the range of a few MHz [7]. The hfs of the $b$ state is unknown, but it could be estimated from the atomic model developed in [8, 9] for $^{39}$KCs, which reveals a manifold of PECs spanning a few MHz at short distances, for the $\Omega = 0$ component of the $b^3\Pi_0$ state relevant for the present study.

Note that in Ref. [10], Karman *et al.* checked in their numerical calculations that the hyperfine structure has no influence on the mw-shielding for a strong enough magnetic field, namely about 100 G in RbCs. In Ref. [11], Lassablière *et al.* elaborated a simple model for all polar molecules, suggesting that for NaRb, the hfs has no influence when the magnetic field is beyond a critical value of 309 G (see Table I of [11]). Therefore the mechanism we describe in our paper is experimentally relevant.

### D. The optical shielding for trapped ultracold molecules

The optical shielding (OS) laser has a wavelength of 884.447 nm. Looking at our results for the NaRb dynamic polarizability curves around 884.5 nm [12], we would need to choose a laser frequency around 66 GHz above the frequency of the transition $X(\nu = 0) \rightarrow b(\nu=0)$ to have the polarizability of the ground-state molecules positive again, and about 150-300 GHz above the same frequency to ensure a trapping strength similar to a typical 1064 nm optical dipole trap. Therefore the shielding laser cannot be used for trapping. An additional trapping laser is needed, which is not considered explicitly in our work. The trapping laser is expected to be responsible for themolecule losses at short distances due to some sort of photoassociation (see [13, 14]). This leads to the definition of $k_{\rm re}$.

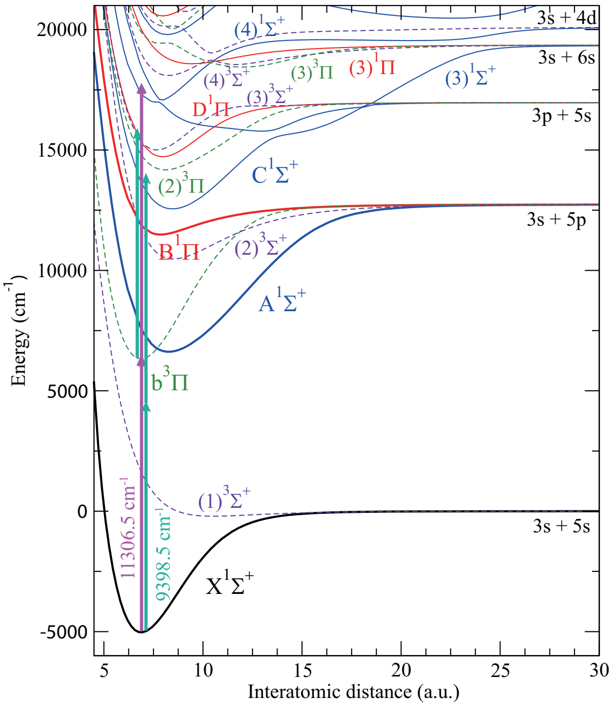


FIG. 4: The Hund's case a potential curves of NaRb [15]. The vertical lines with arrows represent different optical transition processes.

In Fig. 4 We display the relevant Hund's case a PECs of NaRb calculated by us [15]. It is clear that a two-photon transition with the 1064 nm laser (9398.5 cm-1) is very unlikely, as there is no intermediate resonance for the first photon. Also, the $\nu$=0 of the $b^3\Pi$ state could absorb a 1064 nm photon, and the $(3)^3\Sigma^+$ state could be reached in the lower part of its PEC. However, one can

expect that the density of levels will be low enough to avoid any accidental resonance via a fine tuning of the 1064 nm laser.

As above, two-photon transitions with the 884.447 nm (11306.5 cm$^{-1}$) shielding laser are very unlikely: the second photon absorbed the $\nu$=0 level of the $b$ state would reach a zone where no triplet state is present, and would only accidentally be resonant with a bound level there. In terms of Floquet analysis, this means that the Floquet block composed by the $X+X$ asymptote dressed with one photon and the $X+b$ asymptote dressed by zero photon, is lying far outside the energy range which is relevant to our work, namely where the Floquet block composed of the $X+X$ asymptote dressed with zero photon and the $X+b$ asymptote dressed by (-1) photon is located (see Figure 3 of our manuscript). This is certainly in striking contrast with the mw-shielding proposal, for which the detunings are of the same magnitude than the rotational spacings.

### E. Short-range boundary condition in log derivative method

We solve the coupled Schrödinger equations with proper boundary condition starting at short distances. At $R_{min} = 10$ a.u., we initialize the diagonal elements of log-derivative matrix $\mathbb{Z}$ with a complex value for a particular channel $i$ [16],

$$\begin{aligned} \mathbb{Z}_{i,i}(R_{min}) & \\ &= \frac{4k_{min}sc\sqrt{1-p_{SR}}}{c^2(\sqrt{1-p_{SR}}-1)^2+s^2(\sqrt{1-p_{SR}}+1)^2} \\ &\quad -i\frac{k_{min}p_{SR}}{c^2(\sqrt{1-p_{SR}}-1)^2+s^2(\sqrt{1-p_{SR}}+1)^2}, \end{aligned} \quad (1)$$

with

$$k_{min} = \sqrt{\frac{2\mu[E_{tot} - u_{i,i}(R_{min})]}{\hbar^2}}, \quad (2)$$

$$s = \sin(k_{min}R_{min} + \delta_{SR}), \quad (3)$$

$$c = \cos(k_{min}R_{min} + \delta_{SR}). \quad (4)$$

In the above equations, the quantities $0 \leq p_{SR} \leq 1$ and $0 \leq \delta_{SR} \leq \pi$ characterize the probability of flux loss when reaching the short distances, and the phase shift accumulated from the region $R < R_{min}$, respectively. The total energy $E_{tot}$ in the entrance channel slightly differs from the collision energy $E_{col}$, as it includes the energy brought by the electromagnetic field. The diabatic energy $u_{i,i}$ in channel $i$ is the sum of the diagonal element of dipole-dipole interaction in the asymptotically dressed basis set, centrifugal potential term, and the van der Waals term. This formula is deduced after modeling the short range interaction potential by a constant square well with depth $u_{i,i}(R_{min})$ between $R = 0$ and $R_{min}$. With the two parameters $p_{SR}$ and $\delta_{SR}$ we can tune the boundary conditions to simulate different cases. Usually we consider a full loss at short range, with $p_{SR}$ = 1, while $\delta_{SR}$ is arbitrary, so that $\mathbb{Z}(R_{min})$ can be simplified as a pure imaginary value $-ik_{min}$. This model is known as the "universal regime" as no resonance occurs in the scattering length or in the cross section: the results do not depend on the details of the short-range interaction. Due to complex matrix elements in $\mathbb{Z}$, the $S$ matrix is non-unitary, and $1 - |S|^2$ features the chemical reaction probability at short distances.

### F. Optical shielding for other alkali-metal dipolar species

In the main text, we invoked a simple model assuming a scaling of the long-range interaction involving the product of the PDM of the molecular states, and the TDM between the $X$ and $b$ states. In Table III, we collected the relevant data from our own calculations extensively described in [2, 17] for the PDMs and TDMs, and in [3, 4] for the $C_6^{el}$ values. We recall that the latter is taken identical for the $X+X$ and $X+b$ manifolds in our calculations.

We just consider the leading $R^{-3}$ term in dipole-dipole interactions for $X+X$ interactions thus only the permanent dipole moments (PDMs) in the $X$ state are presented [18]. Besides, the TDMs are used to obtain Rabi frequency and field intensities.

We point out that the value of the radiative lifetime of the $b^3\Pi_0(v_b = 0, j_b = 0)$ level is also derived from our calculations [2, 17], and the presentation of these quantities for all alkali-metal dimers will be the subject of a forthcoming publication.

[1] H. Li, G. Quéméner, J.-F. m. c. Wyart, O. Dulieu, and M. Lepers, Phys. Rev. A **100**, 042711 (2019).
[2] M. Aymar and O. Dulieu, J. Chem. Phys. **122**, 204302 (2005).
[3] M. Lepers, R. Vexiau, M. Aymar, N. Bouloufa-Maafa, and O. Dulieu, Phys. Rev. A **88**, 032709 (2013).
[4] R. Vexiau, M. Lepers, M. Aymar, N. Bouloufa-Maafa, and O. Dulieu, J. Chem. Phys. **142**, 214303 (2015).
[5] X. Ye, M. Guo, M. L. González-Martínez, G. Quéméner, and D. Wang, Science Advances **4** (2018).
[6] R. Napolitano, J. Weiner, and P. S. Julienne, Phys. Rev. A **55**, 1191 (1997).
[7] J. Aldegunde and J. M. Hutson, Phys. Rev. A **96**, 042506 (2017).
[8] A. Orbán, R. Vexiau, O. Krieglsteiner, H.-C. Nägerl, O. Dulieu, A. Crubellier, and N. Bouloufa-Maafa, Phys. Rev. A **92**, 032510 (2015).
[9] A. Orbán, T. Xie, R. Vexiau, O. Dulieu, and N. Bouloufa-Maafa, Journal of Physics B: Atomic, Molecular and Optical Physics **52**, 135101 (2019).
[10] T. Karman and J. M. Hutson, Phys. Rev. Lett. **121**, 163401 (2018).
[11] L. Lassablière and G. Quéméner, Phys. Rev. Lett. **121**, 163402 (2018).

| Species | $C_6^{el}$ (a.u.) | $\mathrm{PDM}_X$ (a.u.) | $\mathrm{PDM}_b$ (a.u.) | $\mathrm{TDM}_{X\to b}$ (a.u.) | $B_{(X)}$ ($\mathrm{cm}^{-1}$) | $B_{(b)}$ ($\mathrm{cm}^{-1}$) |
|---|---|---|---|---|---|---|
| $^{7}$Li$^{23}$Na | 3333.6 | 0.2228 | 0.645 | 0.0082 | 0.374 | 0.387 |
| $^{7}$Li$^{39}$K | 6096.8 | 1.410 | 1.810 | 0.0216 | 0.256 | 0.274 |
| $^{7}$Li$^{87}$Rb | 7268 | 1.645 | 2.214 | 0.1149 | 0.215 | 0.231 |
| $^{7}$Li$^{133}$Cs | 9263 | 2.201 | 2.709 | 0.1327 | 0.187 | 0.204 |
| $^{23}$Na$^{39}$K | 7088.1 | 1.095 | 1.220 | 0.0456 | 0.0950 | 0.0951 |
| $^{23}$Na$^{87}$Rb | 8374.6 | 1.304 | 1.735 | 0.1918 | 0.0697 | 0.0700 |
| $^{23}$Na$^{133}$Cs | 10642 | 1.845 | 2.369 | 0.4204 | 0.0579 | 0.0600 |
| $^{39}$K$^{87}$Rb | 12610.1 | 0.2423 | 0.491 | 0.1353 | 0.0378 | 0.0387 |
| $^{39}$K$^{133}$Cs | 15481.9 | 0.7237 | 1.282 | 0.2342 | 0.0304 | 0.0320 |
| $^{87}$Rb$^{133}$Cs | 17839.4 | 0.4903 | 0.840 | 0.2697 | 0.0164 | 0.0170 |

TABLE III: Relevant parameters for transition for the ten species of bosonic alkali-metal diatomics: the electronic part $C_6^{el}$ of the van der Waals interaction (see text), the permanent dipole moments (PDMs) for the $X^1\Sigma(v_X = 0)$ to $b^3\Pi_0(v_b = 0)$ levels, the transition dipole moments (TDMs) between these two levels, their respective rotational constant $B_{(X)}$ and $B_{(b)}$. Both PDM and TDM are displayed in the molecular frame. We recall that 1 a.u.=2.541 580 59 Debye.

[12] R. Vexiau, D. Borsalino, M. Lepers, A. Orbán, M. Aymar, O. Dulieu, and N. Bouloufa-Maafa, Int. Rev. Phys. Chem. **36**, 709 (2017).

[13] A. Christianen, M. W. Zwierlein, G. C. Groenenboom, and T. Karman, Phys. Rev. Lett. **123**, 123402 (2019).

[14] P. D. Gregory, J. A. Blackmore, S. L. Bromley, and S. L. Cornish, Phys. Rev. Lett. **124**, 163402 (2020).

[15] M. Aymar and O. Dulieu, Mol. Phys. **105**, 1733 (2007).

[16] G. Wang and G. Quéméner, New J. Phys. **17**, 035015 (2015).

[17] M. Aymar, O. Dulieu, and F. Spiegelman, J. Phys. B: At. Mol. Opt. Phys. **39**, S905 (2006).

[18] M. Lepers and O. Dulieu, in *Cold Chemistry: Molecular Scattering and Reactivity Near Absolute Zero* (The Royal Society of Chemistry, 2018) pp. 150–202.
